# Supplementary material for: Budgeted Matroid Maximization: a Parameterized Viewpoint
Source: arXiv:2307.04173 source file (2023-07-09)
Supplement: Supplementary file 1 [file appendix.tex]

%\section{Omitted Proofs from Section~\ref{sec:preliminaries}}
%\label{sec:omitted-prel}

\section{Omitted Proofs from Section~\ref{sec:alg}}
\label{sec:omitted-alg}

We give several definitions and claims used in the proof of Lemma~\ref{lem:Solution}. The next general observation follows from applying the exchange property of matroids multiple times. It is used in the proof of Lemma~\ref{ob:matroid}. 
\begin{observation}
	\label{obr:matroid}
	Given a matroid $(E,\cI)$ and $A,B \in \cI$, there is $D \subseteq A \setminus B$, $|D| = \max\{|A|- |B|,0\}$ such that $B \cup D \in  \cI$. 
\end{observation} 
A {\em set system} is a tuple $(E,\cI)$, where $E$ is a ground set of elements and $\cI \subseteq 2^E$ is a set of subsets of $E$ (e.g., a matroid is a set system). A set system $(E,\cI)$ satisfies the {\em hereditary property} if for all $A \in \cI$ and $B \subseteq A$ it holds that $B \in \cI$. Note that the set system $(E,\cm(\cC))$, where $\cC$ is a constraint of $E$, satisfies the hereditary property both for matching constraints and for matroid intersection constraints. %Also, for some $F \subseteq E$ let $\cm \setminus F$ be the contraction of $F$ in the set system $(E,\cm)$. By well-known elementary properties of matroids (matchings), for all $F \subseteq E$, if $\cm$ is a matroid intersection (matching) constraint, then $\cm \setminus F$ is a matroid intersection (matching) constraint, respectively.  
The next result describes a {\em weak exchange property} for both types of constraints. The proof relies on the fact that both matchings and matroid intersection have similar (yet weaker) exchange properties to matroids.%; we give the details in Appendix~\ref{sec:omitted-prel}. %The proof uses that adding an edge (element) to a matching (common independent sets in two matroids)  
\begin{lemma}
	\label{ob:matroid}
	%Given two matroid $M_1 = (E,\cI_1), M_2 = (E,\cI_2)$ and $A,B \in \cI_1 \cap \cI_2$, there is $D \subseteq A \setminus B$, $|D| = \max\{|A|-2 \cdot |B|,0\}$ such that $B \cup D \in  \cI_1 \cap \cI_2$. 
	Given a a ground set $E$, a constraint $\cC$ of $E$, and $A,B \in \cm$, there is $D \subseteq A \setminus B$, $|D| = \max\{|A|-2 \cdot |B|,0\}$ such that $B \cup D \in \cm$. 
\end{lemma}
%\noindent{\bf Proof of Lemma~\ref{ob:matroid}}: 
%We split the proof into two cases based on whether $\cC$ is a matroid constraint or a matching constraint. 
\begin{proof}
	
	Consider the following two cases. \begin{enumerate}
		\item $\cC$ is a matroid intersection constraint. Let $\cC = (\cI_1, \cI_2)$. %There are matroids $(E,\cI_1)$ and $(E, \cI_2)$ such that $\cm =  \cI_1 \cap \cI_2$. 
		By Observation~\ref{obr:matroid}, there are $D_1,D_2 \subseteq A \setminus B$ such that $|D_1| = |D_2| =  \max\{|A| - |B|,0\}$, $B \cup D_1 \in  \cI_1$, and $B \cup D_2 \in  \cI_2$. Observe that $D_1 \cap D_2 \subseteq D_1$ and $D_1 \cap D_2 \subseteq D_2$; hence, by the hereditary properties of $(E,\cI_1)$ and $(E,\cI_2)$ it holds that $B \cup (D_1 \cap D_2) \in  \cI_1 \cap \cI_2 = \cm$. Moreover, \begin{equation*}
			\begin{aligned}
				|D_1 \cap D_2| ={} & |A \setminus \left( (A \setminus D_1) \cup (A \setminus D_2)\right)| \\ \geq{} & |A|-|A \setminus D_1|-|A \setminus D_2| \\ 
				={} & |A|-(|A| - |D_1|)-(|A| - |D_2|) \\ 
				\geq{} & |A|-(|A|-(|A|-|B|))-(|A|-(|A|-|B|)) \\
				={} & |A|- 2 \cdot |B|.
			\end{aligned}
		\end{equation*}
		The first and second equalities hold since $D_1, D_2 \subseteq A$. The second inequality follows from $|D_1| = |D_2| =  \max\{|A| - |B|,0\}$. Hence, we have that $D = D_1 \cap D_2$ satisfies the conditions of the lemma.
		
		\item $\cC$ is a matroid intersection constraint. %There is an undirected graph 
		Let $\cC = (V,E)$ %such that $\cC = G$ and $\cm$ is the set containing all matchings of $G$. 
		and define $D = \{\{u,v\} \in A~|~u,v \notin V(B)\}$. Clearly, $B \cup D$ is a matching of $G$ since $A,B$ are matchings of $G$. In addition, \begin{equation*}
			\begin{aligned}
				|D| ={} & |A \setminus (A \setminus D)| \\
				={} & |A|-\left|\left\{\{u,v\} \in A~|~u \in V(B) \text{ or } v \in V(B)\right\}\right| \\ \geq{} & |A| - |V(B)| \\
				={} & |A|-2 \cdot |B|.
			\end{aligned}
		\end{equation*} The inequality holds since a vertex can be an endpoint in $A$ at most once (recall that $A$ is a matching). The last equality follows by the observation that $|V(B)| = 2 \cdot |B|$, since each edge in a matching has exactly two endpoints, and the endpoints of distinct edges in a matching are disjoint.
	\end{enumerate}
\end{proof}

\noindent{\bf Proof of Lemma~\ref{lem:Solution}}: 
As this proof is based on the proof of a corresponding Lemma in \cite{DKS23}, we use some of their definitions and notations. With a slight abuse of notation, 
we use $\OPT$ to denote an optimal solution for $I$.
Given an optimal solution, we partition a subset of the elements in the solution 
into $\ceil{\eps^{-1}}$ disjoint sets (some sets may be empty). Specifically,
let $N = \ceil{\eps^{-1}}$; for all $i \in [N]$ define 
\begin{equation}
	\label{J_i}
	J_i = \big\{e \in \OPT~\big|~ p(e) \in \big(\eps^{i} \cdot \OPT(I),  \eps^{i-1} \cdot \OPT(I) \big] \big\}.		
\end{equation} 
Let $i^* = \argmin_{i\in [N]} p(J_i)$. By \eqref{J_i} we have at least 
$\eps^{-1}$ disjoint sets; thus, $p(J_{i^*}) \leq \eps \cdot \OPT(I)$. 
Now, let $L~= ~\bigcup_{k \in  [i^*-1]} J_k$ be the subset of all elements in $\OPT$ 
of profits greater than $\eps^{i^*-1} \cdot \OPT(I)$, and $Q = \OPT \setminus (L \cup J_{i^*})$. 
To complete the proof of the lemma, we need several claims.
\begin{claim}
	\label{clam:Iq}
	$L \in \cm_{\leq q(\eps)}$. 
\end{claim}
\begin{claimproof}
	Since $L \subseteq \OPT$, by the hereditary property of $\cm$ we have that $L \in  \cm$. Also, 
	\begin{equation*}
		\label{contradiction1}
		|L| \leq \sum_{e \in L} \frac{p(e)}{\eps^{i^*-1} \cdot \OPT(I)} = \frac{p(L)}{\eps^{i^*-1} \cdot \OPT(I)} \leq  \eps^{- (i^{*}-1)}  \leq   \eps^{-N+1} \leq \eps^{-\eps^{-1}} \leq  q(\eps)
	\end{equation*} The first inequality holds since $p(e) \geq  \eps^{i^*-1} \cdot \OPT$
	for all $e \in L$. For the second inequality, we note that $L$ is a solution for $I$. By the above it follows that $L \in \cm_{\leq q(\eps)}$. 
\end{claimproof} 
By Claim~\ref{clam:Iq} and as $R$ is an SRS,
it follows that $L$ has a replacement $Z_L \subseteq R$. 
Let $\Delta_L = (L \setminus H) \cup Z_L$. By Property~\ref{p:I} of Definition~\ref{def:Replacement}, we have that $\Delta_L \in \cm_{\leq q(\eps)}$, and it also holds that $\cm_{\leq q(\eps)} \subseteq  \cm$. 
Hence, $\Delta_L \in  \cm$. Furthermore, as $Q \subseteq \OPT$ and  $\OPT \in \cm$, by the 
hereditary property for $\cm$ we have that $Q \in  \cm$. Therefore, by Lemma~\ref{ob:matroid}, there is a subset $T \subseteq Q \setminus\Delta_L$, where $|T|  = \max\{|Q| - 2 \cdot |\Delta_L|,0\}$, such that $\Delta_L \cup T \in \cm$. 

Let $S = \Delta_L \cup T$. We show that $S$ satisfies the conditions of the lemma. 

\begin{claim}
	\label{claim:IsSolution}
	$S$ is a solution for $I$. 
\end{claim}

\begin{claimproof}
	By the definition of $T$ it holds that $S = \Delta_L \cup T \in \cm$. Moreover, 	
	\[
	\begin{array}{ll}
		c(S) &= c(\Delta_L\cup T) \\
		& \leq c(Z_L)+ c(L \setminus H) +w(T) \\
		& \leq c(L \cap H)+c(L \setminus H)+c(T) \\ 
		& \leq c(L)+c(Q) \\ 
		& \leq c(\OPT)\\
		& \leq \beta.
	\end{array}
	\]
	The second inequality holds since $c(Z_L) \leq c(L \cap H)$ (see Property~\ref{p:s} of Definition~\ref{def:Replacement}). For the third inequality, recall that $T \subseteq Q$. The last inequality holds since $\OPT$ is a solution for $I$. 
\end{claimproof} 

The proof of the next claim relies on
the {\em profit gap}  between the elements in $Q$ and $L$. 
\begin{claim}
	\label{clam:profitBound1}
	$p\left(Q \setminus T\right) \leq 2\eps \cdot \OPT(I)$.
\end{claim}
\begin{claimproof} 
	
	Observe that 
	\begin{equation}
		\label{eq:menS}
		|Q \setminus T| \leq 2 \cdot |\Delta_L| \leq 2 \cdot |Z_L|+2 \cdot |L \setminus H| \leq 2 \cdot |L \cap H|+2 \cdot |L \setminus H| \leq 2 \cdot |L|.
	\end{equation} 
	The first inequality follows from the definition of $T$. For the third inequality, we use Property~\ref{p:car} of Definition~\ref{def:Replacement}. Hence, 
	\begin{equation*}
		\begin{aligned}
			p(Q \setminus T) \leq{} & |Q \setminus T| \cdot \eps^{i^*} \cdot \OPT(I) \leq  2 \cdot |L| \cdot \eps^{i^*} \cdot \OPT(I) \leq 2\eps \cdot p(L) \leq 2\eps \cdot \OPT(I).
		\end{aligned}
	\end{equation*} 
	
	The first inequality holds since $p(e) \leq \eps^{i^*} \cdot \OPT(I)$ for all $e \in Q$. 
	The second inequality is by \eqref{eq:menS}. The third inequality holds since $p(e) > \eps^{i^*-1} \cdot \OPT(I)$ for all $e \in L$. 
\end{claimproof} 	

\begin{claim}
	\label{clam:profitBound2}
	$p\left(S\right) \geq (1-4\eps) \OPT(I)$.
\end{claim} 

\begin{claimproof} 
	By Property~\ref{p:p} of Definition~\ref{def:Replacement},
	\begin{equation}
		\label{eq:proofProfit1}
		\begin{aligned}
			p(\Delta_L) ={} & p((L \setminus H) \cup Z_L) \geq (1-\eps) \cdot p(L).
		\end{aligned}
	\end{equation} Moreover, 
	\begin{equation}
		\label{eq:proofProfit2}
		\begin{aligned}
			p(T) {} & \geq p(Q) - p(Q \setminus T) \geq p(Q) - 2\eps \cdot \OPT(I) \geq (1-\eps) \cdot p(Q) - 2\eps \cdot \OPT(I). 
		\end{aligned}
	\end{equation} 
	
	The second inequality is by Claim~\ref{clam:profitBound1}. Using \eqref{eq:proofProfit1} and \eqref{eq:proofProfit2}, we have that 
	
	\[	
	\begin{array}{ll}
		p(\Delta_L)+p(T) & \geq (1-\eps) \cdot p(L \cup Q)-2\eps \cdot \OPT(I) 
		\\ & = (1-\eps) \cdot p(\OPT \setminus J_{i^*})-2\eps \cdot \OPT(I) \\
		&  \geq (1-\eps) \cdot (1-\eps) \cdot \OPT(I)-2\eps \cdot \OPT(I)\\
		&  \geq (1-4\eps) \cdot \OPT(I). 
	\end{array}
	\]
	
	The second inequality holds since $p(J_{i^*}) \leq \eps \cdot \OPT(I)$. Observe that 
	$S = \Delta_L \cup T$ and $T \cap \Delta_L = \emptyset$. Therefore,  $$p(S) = p(\Delta_L)+p(T) \geq (1-4\eps) \cdot \OPT(I).$$
	
\end{claimproof} 
Finally, we note that, by \eqref{J_i} and the definition of $Q$, it holds that $Q \cap H = \emptyset$. Consequently, by the definition of $S$, we have that $S \cap H \subseteq Z_L$. 
As $Z_L \subseteq R$ (by Definition~\ref{def:Representatives}), it follows that $S \cap H \subseteq R$. Hence, using Claims~\ref{claim:IsSolution} and~\ref{clam:profitBound2}, it follows that $R$ is a representative set by Definition~\ref{def:REP}.
%we have the statement of the lemma.  \qed
%%%%%%%%%%%%%%%%%%%%%%%%%%%%%%%%%%%%%%%%%%%%%%%%%%%%%%%%%%%%%%%%

{\bf Proof of Lemma~\ref{lem:sufficientRep}:}
	For the proof of the lemma, we define a {\em substitution} of some feasible set adapting the definition in \cite{DKS23}. The first two properties of substitution of some $G \in \cm_{\leq q(\eps)}$ are identical to the first two properties in the definition of a replacement of $G$. 
	However, we require that a substitution preserves the number of profitable elements in $G$ from each profit class, and that a substitution must be disjoint to the set of non-profitable elements in $G$. %
	
	\begin{definition}
		\label{def:sub}
		For $G \in \cm_{\leq q(\eps)}$ and $Z_G \subseteq \bigcup_{r \in [\log_{1-\eps} \left(\frac{\eps}{2}\right)+1] } {\ck}_r(\alpha)$, we say that $Z_G$ is a {\em substitution} of $G$ if the following holds. \begin{enumerate}

			\item $(G \setminus H) \cup Z_G \in \cm_{\leq q(\eps)}$.\label{pp:1}
			
			\item  $c(Z_G) \leq c(G \cap H)$.\label{pp:2}
			
			\item For all $r \in [\log_{1-\eps} \left(\frac{\eps}{2}\right)+1]$ it holds that $|{\ck}_r(\alpha) \cap Z_G| = |{\ck}_r(\alpha) \cap G \cap H|$.\label{pp:3}

			\item $(G \setminus H) \cap Z_G = \emptyset$.\label{pp:4}
		\end{enumerate}
	\end{definition}
	\begin{claim}
		\label{claim:substitution}
		For any $G \in \cm_{\leq q(\eps)}$ there is a substitution $Z_G$ of $G$ such that $Z_G \subseteq R$. 
	\end{claim}
	\begin{claimproof}
		Let $G \in \cm_{\leq q(\eps)}$ and let $Z_G$ be a substitution of $G$ such that $|Z_G \cap R|$ is maximal among all substitutions of $G$; formally, let $\mathcal{S}(G)$ be all substitutions of $G$ and let $Z_G \in \{ Z \in \mathcal{S}(G)~|~ |Z \cap R| = \max_{Z' \in \mathcal{S}(G)} |Z' \cap R|\}$. Since $G \cap H$ is in particular a substitution of $G$  it follows that $\mathcal{S}(G)\neq \emptyset$, and thus  $Z_G$ is well defined.  Assume towards a contradiction that there is $a \in Z_G \setminus R$; then, by Definition~\ref{def:sub} there is $r \in [\log_{1-\eps} \left(\frac{\eps}{2}\right)+1]$ such that $a \in {\ck}_r(\alpha)$. Let $\Delta_G = (G \setminus H) \cup Z_G$; by definition~\ref{def:sub} it holds that $\Delta_G \in \cm_{\leq q(\eps)}$. In addition, because $R$ is exchange for $I,\eps,\alpha$, and $r$, by Definition~\ref{def:r-set} there is $b \in ({\ck}_r(\alpha) \cap R) \setminus \Delta_G$ such that $c(b) \leq c(a)$ and $\Delta_G -a+b \in \cm_{\leq q(\eps)}$. Then,  the properties of Definition~\ref{def:sub} are satisfied for $Z_G-a+b$ by the following. 
		\begin{enumerate}
			\item $(G\setminus H) \cup (Z_G -a +b) =  \Delta_G-a+b \in \cm_{\leq q(\eps)}$ by the definition of $b$. 
			
			\item  $c(Z_G-a+b) \leq c(Z_G) \leq c(G\cap H)$ because $c(b) \leq c(a)$. 
			
			\item for all $r' \in [\log_{1-\eps} \left(\frac{\eps}{2}\right)+1]$ it holds that $|{\ck}_{r'}(\alpha) \cap (Z_G-a+b)| = |{\ck}_{r'}(\alpha) \cap Z_G| = |{\ck}_{r'}(\alpha) \cap G \cap H|$ because $a,b \in {\ck}_r(\alpha)$.
			
			\item $|(G \setminus H) \cap (Z_G -a+b)| \leq |(G \setminus H) \cap (Z_G)| = 0$ where the inequality follows because $b \notin \Delta_G$ and the equality is since $Z_G$ is a substitution of $G$. 
		\end{enumerate}
		
		By the above and Definition~\ref{def:sub}, it follows that $Z_G+a-b$ is a substitution of $G$; that is, $Z_G+a-b \in \mathcal{S}(G)$. Moreover, \begin{equation}
			\label{eq:ZG}
			|R \cap (Z_G -a+b)|>|R \cap Z_G| = \max_{Z \in \mathcal{S}(G)} |Z \cap R|.
		\end{equation} The first inequality is because $a \in Z_G \setminus R$ and $b \in R$. By \eqref{eq:ZG} we reach a contradiction since we found a substitution of $G$ with more elements in $R$ than $Z_G \in \mathcal{S}(G)$, which is defined as a substitution of $G$ with maximal number of elements in $R$. Therefore, $Z_G \subseteq R$ as required.
		\end{claimproof}
	 %$Z_G \in \mathcal{S}(G)$. 
	%

\begin{claim}
	\label{claim:RR}
	For all $e \in H$ such that $\{e\} \in \cm$, there is exactly one $r \in [\log_{1-\eps} \left(\frac{\eps}{2}\right)+1]$ such that $e \in {\ck}_r(\alpha)$.
\end{claim}
\begin{claimproof}
	Let $e \in H$. Observe that: \begin{equation}
		\label{eq:app}
		\frac{\eps}{2} \leq \frac{p(e)}{2 \cdot \OPT(I)} \leq \frac{p(e)}{2 \cdot \alpha} \leq \frac{p(e)}{\OPT(I)} \leq 1.
	\end{equation}The first inequality holds since $e \in H$. The second and third inequalities follow since
	$\frac{\OPT(I)}{2} \leq \alpha \leq \OPT(I)$. The last inequality is because $\{e\}$ is a solution of $I$ (or this element can be discarded from the instance as it cannot appear in any solution of $I$). In addition, observe that for $r_0 = \ceil{\log_{1-\eps} \frac{\eps}{2}}$ it holds that $(1-\eps)^{r_0} \leq \frac{\eps}{2}$ and that for $r_1 = 1$ it holds that $(1-\eps)^{r_1-1} = 1$. Hence, because $r_0 \leq \floor{\log_{1-\eps} \left(\frac{\eps}{2}\right)+1}$, by \eqref{eq:app}, there is exactly one $r \in [\log_{1-\eps} \left(\frac{\eps}{2}\right)+1]$ such that $\frac{p(e)}{2\alpha} \in \big((1-\eps)^r, (1-\eps)^{r-1}\big]$; thus, by \eqref{Er} it holds that $e \in {\ck}_r(\alpha)$ and $e \notin {\ck}_{r'}(\alpha)$ for $r' \in [\log_{1-\eps} \left(\frac{\eps}{2}\right)+1] \setminus \{r\}$.  
\end{claimproof}

 The proof of Lemma~\ref{lem:sufficientRep} follows by showing that for any $G \in \cm_{\leq q(\eps)}$ a substitution of $G$ which is a subset of $R$ is in fact a replacement of $G$. Let $G \in \cm_{\leq q(\eps)}$; by Claim~\ref{claim:substitution}, $G$ has a substitution $Z_G \subseteq R$. Then, \begin{equation}
	\label{eq:profitR}
	\begin{aligned}
		p(Z_G) \geq{} & \sum_{r \in [\log_{1-\eps} \left(\frac{\eps}{2}\right)+1]} p({\ck}_r(\alpha) \cap Z_G) 
		\\ \geq{} &  \sum_{r \in [\log_{1-\eps} \left(\frac{\eps}{2}\right)+1] \text{ s.t. } {\ck}_r(\alpha) \neq \emptyset} |{\ck}_r(\alpha) \cap Z_G| \cdot \min_{e \in {\ck}_r(\alpha)} p(e) 
		\\ \geq{} & \sum_{r \in [\log_{1-\eps} \left(\frac{\eps}{2}\right)+1] \text{ s.t. } {\ck}_r(\alpha) \neq \emptyset} |{\ck}_r(\alpha) \cap G \cap H| \cdot (1-\eps) \cdot \max_{e \in {\ck}_r(\alpha)} p(e) 
		\\ \geq{} & (1-\eps) \cdot p(G \cap H).
	\end{aligned}
\end{equation}  The third inequality is by \eqref{Er} and by Property~\ref{pp:3} of Definition~\ref{def:sub}. The last inequality follows from Claim~\ref{claim:RR} (note that $\{e\} \in \cm$ for all $e \in G \cap H$ by the hereditary property). Therefore,  
\begin{equation}
	\label{eq:profitFINAL}
	\begin{aligned}
		p((G \setminus H) \cup Z_G) & = p(G \setminus H)+p(Z_G) \\
		&  \geq p(G \setminus H)+(1-\eps) \cdot p(G \cap H) \\
		& \geq (1-\eps) \cdot p(G).
	\end{aligned}
\end{equation}
The first equality follows from Property~\ref{pp:4} of Definition~\ref{def:sub}. The first inequality is by \eqref{eq:profitR}. Now,  $Z_G$ satisfies Property~\ref{p:I} and~\ref{p:s} of Definition~\ref{def:Replacement} by Properties~\ref{pp:1},~\ref{pp:2} of Definition~\ref{def:sub}, respectively. In addition, $Z_G$ satisfies Property~\ref{p:p} of Definition~\ref{def:Replacement} by \eqref{eq:profitFINAL}. Finally, $Z_G$ satisfies Property~\ref{p:car}  of Definition~\ref{def:Replacement} by 
$$|Z_G| = \sum_{r \in [\log_{1-\eps} \left(\frac{\eps}{2}\right)+1]} |Z_G \cap {\ck}_r(\alpha)| \leq \sum_{r \in [\log_{1-\eps} \left(\frac{\eps}{2}\right)+1]} |G \cap H \cap {\ck}_r(\alpha)| = |G \cap H|.$$ 
The first inequality holds since $Z_G$ is a substitution of $G$. The last equality follows from Claim~\ref{claim:RR}. We conclude that $Z_G$ is a replacement of $G$ such that $Z_G \subseteq R$; thus, $R$ is a strict representative set by Definition~\ref{def:Representatives}. Therefore, it follows that $R$ is a representative set by Lemma~\ref{lem:Solution}. \qed

	In the following proofs we rely on the next technical auxiliary claim. \begin{claim}
	\label{claim:log}
	For all $0<\eps<\frac{1}{2}$ it holds that $\log_{1-\eps} \left(\frac{\eps}{2}\right)+1 \leq 3 \eps^{-2}$.
\end{claim}
\begin{claimproof}
	Using logarithm rules we have
	\begin{equation*}
		\label{eq:log1}
		\log_{1-\eps} \left(\frac{\eps}{2}\right)+1  \leq 
		\frac{\ln \left(\frac{2}{\eps}\right)}{-\ln \left(1-\eps \right)}+1 \leq \frac{2\eps^{-1}}{\eps}+1 \leq 3 \eps^{-2}. 
	\end{equation*} 
	The second inequality follows from  $x< -\ln (1-x), \forall x>-1, x \neq 0$, and $\ln (y) < y, \forall y>0$. 
\end{claimproof}

\noindent
{\bf Proof of Lemma~\ref{lem:main}:}
	Let $\alpha$ be the result of Step~\ref{step:REPalpha} of Algorithm~\ref{alg:findRep} and $r \in  [\log_{1-\eps} \left(\frac{\eps}{2}\right)+1]$. We distinguish between two cases, depending on the type of constraint. 
	\begin{itemize}
		\item 	If $I$ is a BM instance then, by Lemma~\ref{lem:mainMatching}, $ \textsf{ExSet-Matching}(I,\eps,\alpha,r)$ is an exchange set for $I,\eps,\alpha$, and $r$ such that $\left|     \textsf{ExSet-Matching}(I,\eps,\alpha,r)    \right| \leq 18 \cdot {q(\eps)}^2$. Therefore %by
		%Algorithm~\ref{alg:findRep}, 
	  $R \cap {\ck}_r(\alpha)$ is an exchange set for $I,\eps,\alpha$, for all $r \in  [\log_{1-\eps} \left(\frac{\eps}{2}\right)+1]$ and \begin{equation*}
	  	|R| \leq \left( \log_{1-\eps} \left(\frac{\eps}{2}\right)+1\right)  \cdot 18 \cdot q(\eps)^2 \leq 3 \cdot \eps^{-2} \cdot 18 \cdot q(\eps)^2 \leq 54 \cdot {q(\eps)}^3. 
	  \end{equation*}  The second inequality follows from Claim~\ref{claim:log}. Then, by Lemma~\ref{lem:sufficientRep}, $R$ is a representative set of $I$ and~$\eps$; furthermore, $|R| \leq 54 \cdot {q(\eps)}^3$. 
		
		As for the running time, observe that Step~\ref{step:REPAPP} can be computed in time $\textnormal{poly}(|I|)$ using a PTAS for BC with
		an error parameter $\eps= \frac{1}{2}$ (see~\cite{BBGS11}). In addition, each iteration of the \textbf{for} loop of Step~\ref{step:REPforr} can be computed in time $q(\eps) \cdot \textnormal{poly}(|I|)$ by Lemma~\ref{lem:mainMatching}. Hence, as we have $\left(\log_{1-\eps} \left(\frac{\eps}{2}\right)\right)+1$ iterations of the  \textbf{for} loop of Step~\ref{step:REPforr} , the running time of the algorithm is bounded by $$ \left( \log_{1-\eps} \left(\frac{\eps}{2}\right)+1\right)  \cdot q(\eps) \cdot  \textnormal{poly}(|I|) \leq 6 \cdot \eps^{-2} \cdot q(\eps) \cdot  \textnormal{poly}(|I|) \leq q(\eps)^2 \cdot \textnormal{poly}(|I|).$$ The first inequality follows from Claim~\ref{claim:log}. %We show more rigorously that $\log_{1-\eps} \left(\frac{\eps}{2}\right) +1 \leq 3 \cdot \eps^{-2}$ in Appendix~\ref{sec:omitted-alg}. 
		%Thus, it follows that $|R| \leq 3 \cdot \eps^{-2} \cdot 18 \cdot q(\eps)^2 \leq 54 \cdot {q(\eps)}^3$.
		\item  If $I$ is a BI instance, then by Lemma~\ref{lem:mainMatroid}, $\textsf{ExSet-MatroidIntersection}(I,\eps,\alpha,r)$ is an exchange set for $I,\eps,\alpha$, and $r$ such that $\left|     \textsf{ExSet-MatroidIntersection}(I,\eps,\alpha,r)    \right| \leq {q(\eps)}^{O(q(\eps))}$. Therefore, by Step~\ref{step:REPforr}, Step~\ref{step:matroid}, and Step~\ref{step:REPret} of Algorithm~\ref{alg:findRep} it holds that $R$ is an exchange set for $I,\eps,\alpha$, for all $r \in  [\log_{1-\eps} \left(\frac{\eps}{2}\right)+1]$ such that $|R| \leq \left( \log_{1-\eps} \left(\frac{\eps}{2}\right)+1\right)  \cdot  {q(\eps)}^{O(q(\eps))}$.  Then, by Definition~\ref{def:r-set} and Lemma~\ref{lem:sufficientRep} it holds that $R$ is a representative set of $I$ and $\eps$. 
		
		Observe that Step~\ref{step:REPAPP} can be computed in time $\textnormal{poly}(|I|)$ using a PTAS for BC with
		an error parameter $\eps= \frac{1}{2}$ (see~\cite{BBGS11}). In addition, each iteration of the \textbf{for} loop of Step~\ref{step:REPforr} can be computed in time ${q(\eps)}^{O(q(\eps))} \cdot \textnormal{poly}(|I|)$ by Lemma~\ref{lem:mainMatroid}. Hence, as we have $O\left(\log_{1-\eps} \left(\frac{\eps}{2}\right)\right) $ iterations of the  \textbf{for} loop of Step~\ref{step:REPforr}, the running time of the algorithm is $O\left(\log_{1-\eps} \left(\frac{\eps}{2}\right)\right)  \cdot {q(\eps)}^{O(q(\eps))} \cdot \textnormal{poly}(|I|)$; then, by Claim~\ref{claim:log} it holds that $O\left(\log_{1-\eps} \left(\frac{\eps}{2}\right)\right) = O(\eps^{-2})$ and it follows that $O\left(\log_{1-\eps} \left(\frac{\eps}{2}\right)\right)  = {q(\eps)}^{O(1)}$. Thus, the running time of the algorithm is $ {q(\eps)}^{O(q(\eps))} \cdot \textnormal{poly}(|I|)$. In addition, since $O\left(\log_{1-\eps} \left(\frac{\eps}{2}\right)\right) = O(\eps^{-2})$ by Claim~\ref{claim:log}, it follows that $|R| \leq {q(\eps)}^{O(q(\eps))}$.
	\end{itemize}  \qed

 %The proof of the complementary case, where $I$ is a BI instance, is similar. %We give the details in Appendix~\ref{sec:omitted-alg}.

%{\bf Proof of Lemma~\ref{lem:main}:}
	%Let $\alpha$ be the result of Step~\ref{step:REPalpha} of Algorithm~\ref{alg:findRep} and let $r \in  [\log_{1-\eps} \left(\frac{\eps}{2}\right)+1]$. We complete the proof from Section~\ref{sec:alg} for the complementary case where $I$ is a BI instance. 
		%
		%$\cC$ is a matroid intersection constraint. 
		
	%\end{itemize}

For the proof of Lemma~\ref{thm:EPTAS}, we use the next auxiliary lemmas.  

\begin{lemma}
	\label{thm:aux1}
	Given a \textnormal{BC} instance $I = (E, \cC, c,p, \beta)$ and $0<\eps<\frac{1}{2}$, Algorithm~\ref{alg:EPTAS} returns a solution for $I$ of profit at least $(1-8\eps) \cdot \OPT(I)$.
\end{lemma}

\begin{proof}

	By Lemma~\ref{lem:main} it holds that $R = \textsf{RepSet}(I,\eps)$ is a representative set of $I$ and $\eps$. Therefore, by Definition~\ref{def:REP} there is a solution $S$ for $I$ such that $S \cap H \subseteq R$, and \begin{equation}
		\label{eq:profitS}
		p\left(S\right) \geq (1-4\eps) \cdot \OPT(I).
	\end{equation} As for all $e \in S \cap H$ we have $p(e) > \eps \cdot \OPT(I)$, and $S$ is a solution for $I$, it follows that $|S \cap H| \leq \eps^{-1}$.
	% Then, by Step~\ref{step:for} of Algorithm~\ref{alg:EPTAS} 
	We note that there is an iteration of Step~\ref{step:for} in which $F = S \cap H$; thus, in Step~\ref{step:vertex} we construct a solution $T_{S \cap H}$ of $I_{S \cap H}$ such that: %We use $X(A) = \{e \in E(\alpha) \setminus A~|~ \bar{\lambda}^{A}_e = 1\}$ for every basic solution $\bar{\lambda}^{A}$ computed in Step~\ref{step:vertex} for $A \subseteq R$.  
	\begin{equation}
		\label{eq:finalProfitA}
		\begin{aligned}
			p\left(T_F\right) \geq{} & \OPT(I_{S \cap H})-2 \cdot \max_{e \in E_{S \cap H}} p(e) \\
			\geq{} & p(S \setminus H)- 2 \cdot \max_{e \in E_{S \cap H}} p(e) \\
			\geq{} & p(S \setminus H)-4\eps \cdot \OPT(I). 
		\end{aligned}
	\end{equation}
	%The first inequality holds since $S \setminus H$ is in particular a solution of the extension instance $I_F(\alpha)$ by Definition~\ref{def:instance}. 
	The first inequality holds by Lemma~\ref{lem:grandoni}. The second inequality holds since $S \setminus H$ is in particular a solution of the residual instance $I_F(\alpha)$ by Definition~\ref{def:instance}. The third inequality holds since for all $e \in E_{S \cap H}$ it holds that $p(e) \leq 2\eps \cdot \alpha \leq 2 \eps \cdot \OPT(I)$. Now, recall that $K_{S \cap H}$ defined in Step~\ref{step:Cf} of Algorithm~\ref{alg:EPTAS}. 
	\begin{equation}
		\label{eq:finalProfit}
		\begin{aligned}
			p(K_{S \cap H}) ={} & p(S \cap H)+p\left(T_F\right)  \geq  p(S)- 4\eps \cdot \OPT(I) \geq (1-8\eps) \cdot \OPT(I).
		\end{aligned}
	\end{equation}
	
	The first inequality uses~\eqref{eq:finalProfitA}. The last inequality is by \eqref{eq:profitS}.  \begin{claim}
		\label{claim:Cf}
		$A  = \textnormal{\textsf{EPTAS}}(\cI,\eps)$ is a solution of $I$. 
	\end{claim}
	\begin{claimproof} If $A = \emptyset$ the claim trivially follows since $\emptyset$ is a solution of $I$. Otherwise, by Step~\ref{step:update} of Algorithm~\ref{alg:EPTAS}, there is a solution $F$ of $I$ such that $A = K_F$. Thus, in this case $A$ is a solution for $I$ by Observation~\ref{ob:residual}.
	\end{claimproof} 
	
	By Claim~\ref{claim:Cf}, Steps~\ref{step:for}, \ref{step:update} and~\ref{step:retA}
	of Algorithm~\ref{alg:EPTAS} and \eqref{eq:finalProfit}, we have that
	$A = \textsf{EPTAS}(I,\eps)$ is a solution for $I$ satisfying $p(A) \geq p(K_{S \cap H}) \geq (1-8\eps) \OPT(I)$. This completes the proof. 	
\end{proof}

\begin{lemma}
	\label{thm:aux2}
	Given a \textnormal{BC} instance $I = (E, \cC, c,p, \beta)$ and $0<\eps<\frac{1}{2}$, the running time of Algorithm~\ref{alg:EPTAS} satisfies one of the following. \begin{itemize}
		
			\item If $I$ is a \textnormal{BM} instance  the running time is $2^{ O \left(\eps^{-2} \log \frac{1}{\eps} \right)} \cdot \textnormal{poly}(|I|)$.
		
		\item If $I$ is a \textnormal{BI} instance the running time is ${q(\eps)}^{O(\eps^{-1} \cdot q(\eps))} \cdot \textnormal{poly}(|I|)$.

	\end{itemize}
\end{lemma}
\begin{proof}

	In the following, let $W' = \big\{F \subseteq R~\big|~ |F| \leq \eps^{-1}, F \in \cm(\cC), c(F) \leq \beta\big\}$ be all feasible sets considered in Step~\ref{step:for} of Algorithm~\ref{alg:EPTAS} and let $W = \big\{F \subseteq R~\big|~ |F| \leq \eps^{-1}\big\}$. Observe that the number of iterations of Step~\ref{step:for} of Algorithm~\ref{alg:EPTAS} is bounded by $|W|$, since $W' \subseteq W$ and for each $F \in W$ we can verify in polynomial time if $F \in W'$. We split the analysis for the upper bound on $|W|$ into two parts. \begin{enumerate}

		\item 	$I$ is a BM instance. %By Lemma~\ref{lem:main}, the time complexity of Step~\ref{step:rep} 
		%
		%is $q(\eps) \cdot \textnormal{poly}(|I|)$. Step~\ref{step:APP2} can be computed in time $\textnormal{poly}(|I|)$, by using a PTAS for BC taking 
		%with parameter 
		%$\eps=\frac{1}{2}$ (see~\cite{BBGS11}). 

		\begin{equation}
			\label{eq:subR}
			\begin{aligned}
				|W| \leq{} &  \left(|R|+1\right)^{\eps^{-1}}\\
				\leq{} &  \left(54 \cdot {q(\eps)}^3+1\right)^{\eps^{-1}} \\ 
				\leq{} & {\left(\eps^{-6}\right)}^{\eps^{-1}} \cdot \ceil{\eps^{-\eps^{-1}}}^{3 \cdot \eps^{-1}} \\
				\leq{} & {\eps^{-6 \cdot \eps^{-1}-6\eps^{-2}}} \\
				={} & 2^{ O \left(\eps^{-2} \log \frac{1}{\eps} \right)}.
			\end{aligned}
		\end{equation} %The second inequality is by \eqref{eq:R}. 
	The second inequality holds by Lemma~\ref{lem:main}. The third inequality holds since $0<\eps<\frac{1}{2}$. %Hence, by \eqref{eq:subR}, the number of iterations of the {\bf for} loop  in Step~\ref{step:for} is bounded by $2^{ O \left(\eps^{-2} \log \frac{1}{\eps} \right)}$. In addition, by Lemma~\ref{lem:grandoni}, the running time of each iteration is  $\textnormal{poly}(|I|)$. By the above, the running time of Algorithm~\ref{alg:EPTAS} is $2^{ O \left(\eps^{-2} \log \frac{1}{\eps} \right)} \cdot \textnormal{poly}(|I|)$   if $I$ is a matching-BC instance.

		\item $I$ is a BI instance. 
		%By Lemma~\ref{lem:main}, the time complexity of Step~\ref{step:rep} 
	%
	%	is ${q(\eps)}^{O(q(\eps))}  \cdot \textnormal{poly}(|I|)$. In addition, Step~\ref{step:APP2} can be computed in time $\textnormal{poly}(|I|)$, by using a PTAS for BC taking 
	%with parameter 
	%	$\eps=\frac{1}{2}$ (see~\cite{BBGS11}). 
	% Now, Let $$W = 	\big\{F \subseteq R~\big|~ |F| \leq \eps^{-1}, F \in \cm(\cC), c(F) \leq \beta\big\}$$ be the set of solutions considered in Step~\ref{step:for} of Algorithm~\ref{alg:EPTAS}. 
	Then,
	\begin{equation}
		\label{eq:subR11111}
		\begin{aligned}
			|W| \leq{} &  \left(|R|+1\right)^{\eps^{-1}}
			\leq  {\left({q(\eps)}^{O(q(\eps))}\right)}^{\eps^{-1}} = {q(\eps)}^{O(\eps^{-1} \cdot q(\eps))}.
		\end{aligned}
	\end{equation} 
	The second inequality follows from Lemma~\ref{lem:main}. %Hence, by \eqref{eq:subR11111}, the number of iterations of the {\bf for} loop  in Step~\ref{step:for} is bounded by ${q(\eps)}^{O(\eps^{-1} \cdot q(\eps))}$. In addition, by Lemma~\ref{lem:grandoni}, the running time of each iteration is  $\textnormal{poly}(|I|)$. By the above, the running time of Algorithm~\ref{alg:EPTAS} is ${q(\eps)}^{O(\eps^{-1} \cdot q(\eps))} \cdot \textnormal{poly}(|I|)$  if $I$ is a matroid-BC instance.

	\end{enumerate} Hence, by \eqref{eq:subR} and \eqref{eq:subR11111}, the number of iterations of the {\bf for} loop  in Step~\ref{step:for} is bounded by $2^{ O \left(\eps^{-2} \log \frac{1}{\eps} \right)}$ and ${q(\eps)}^{O(\eps^{-1} \cdot q(\eps))}$ for BM and BI instances, respectively. In addition, by Lemma~\ref{lem:grandoni}, the running time of each iteration is  $\textnormal{poly}(|I|)$. By the above, the running time of Algorithm~\ref{alg:EPTAS} is $2^{ O \left(\eps^{-2} \log \frac{1}{\eps} \right)} \cdot \textnormal{poly}(|I|)$ if $I$ is a BM instance, and the running time is ${q(\eps)}^{O(\eps^{-1} \cdot q(\eps))} \cdot \textnormal{poly}(|I|)$  if $I$ is a BI instance.  \end{proof} 

%By the above, the proof of Lemma~\ref{thm:EPTAS} follows.

\noindent{\bf Proof of Lemma~\ref{thm:EPTAS}:} The proof follows from Lemma~\ref{thm:aux1} and Lemma~\ref{thm:aux2}. \qed

\section{Omitted Proofs from Section~\ref{sec:lemMainProofMatching}}
\label{sec:omitted-match}

%{\bf Proof of Claim~\ref{claim:elementaryM}:} \begin{claimproof} Observe that $M$ is initialized to be a (empty) matching of $G$ in Step~\ref{step:greedy:init}. In addition, if $M$ is a matching of $G$ at Step~\ref{step:greedy:while} of some iteration, then for any $e \in E / M$ it holds that $M+e$ is a matching of $G$ by the definition of the thinning $E / M$ of $M$ on $E$. Hence, we conclude that by Step~\ref{step:greedy:update} and Step~\ref{step:greedy:return} Algorithm~\ref{alg:greedyMatching} returns a matching of $G$. For the running time, in each iteration of the {\bf while} loop in Step~\ref{step:greedy:while} an edge $e \in E / M$ is added to $M$ by Step~\ref{step:greedy:e}   and Step~\ref{step:greedy:update}. Therefore, because $E / M$ is disjoint from $M$ by the definition of $E / M$, we conclude that in each iteration of the {\bf while} loop in Step~\ref{step:greedy:while} the cardinality of $M$ increases; hence, the number of iterations is bounded by $|E|$. Moreover, each iteration takes a linear time by iterating over all edges in $E / M$ (at most) in Step~\ref{step:greedy:e}, and overall the running time is polynomial. \end{claimproof}

{\bf Proof of Claim~\ref{claim:RunningMatch}:} For the running time, observe that each iteration of the {\bf for} loop of Step~\ref{step:match:for} can be computed in polynomial time, since Step~\ref{step:mathc:Gi} and Step~\ref{step:match:Update} take linear time and Step~\ref{step:match:M} takes polynomial time by Lemma~\ref{lem:GreedyMatching}. Thus, as we have $k(\eps)  = O(q(\eps))$ iterations, the running time is $q(\eps) \cdot \textnormal{poly}(|I|)$. Finally, for the size of the exchange set $X$: \begin{equation*}
	|X| = \left|  \bigcup_{i \in [k(\eps)]} M_i \right| \leq \sum_{i \in [k(\eps)]} |M_i| \leq k(\eps) \cdot N(\eps) = 18 \cdot q(\eps)^2. 
\end{equation*}The first equality holds by Step~\ref{step:match:Update} and Step~\ref{step:match:return}. The second inequality holds since $\forall i \in [k(\eps)]:~|M_i| \leq N(\eps)$ by Lemma~\ref{lem:GreedyMatching}. The last equality holds since $k(\eps) = 2 \cdot N(\eps) = 6 \cdot q(\eps)$. \qed

%%%%%%%%%%%%%%%%%%%%%%%%%%%%%%%%%%%%%%%%%%%%%%%%%%%%%%

\section{Omitted Proofs from Section~\ref{sec:lemMainProof}}
\label{sec:omitted-matroid}

%We use %Lemma~\ref{lem:gen} and 
Lemmas~\ref{lem:notIS} and \ref{lem:gen} provide basic matroid properties used in this section; %in this section;  %the proof of Lemma~\ref{lem:Thereb}; 
the proofs can be found in \cite{DKS23}. 
%\begin{lemma}
	%\label{lem:gen}
	%Let $ (E,\cI)$ be a matroid, $A,B \in \cI$, and $a \in A \setminus B$ such that $B+a \notin \cI$. Then there is $b \in B \setminus A$ such that $A-a+b \in \cI$. 
%\end{lemma}

%The next lemma gives a general property of minimum bases of matroids.
\begin{lemma}
	\label{lem:notIS}
	Given a matroid $(E,\cI)$ and a cost function $c:E \rightarrow \mathbb{R}_{\geq 0}$, let $B$ be a minimum basis of $(E,\cI)$ w.r.t. $c$. Then, for any $a \in E \setminus B$ it holds that $\{e\in B ~|~ c(e)\leq c(a)\}+ a \notin \cI$. 	 
\end{lemma}

%In the proof of Lemma~\ref{lem:maximum} we use the following 
%We use in the proof the next 
%general property of matroids (see the proof, e.g., in~\cite{DKS23}). 
\begin{lemma}
	\label{lem:gen}
	Let $ (E,\cI)$ be a matroid, $A,B \in \cI$, and $a \in A \setminus B$ such that $B+a \notin \cI$. Then there is $b \in B \setminus A$ such that $A-a+b \in \cI$. 
\end{lemma} 

We give a more general formulation of Lemma~\ref{lem:Thereb}. 
\begin{lemma}
	\label{lem:NN}
 Let $\cG = (E,\cI)$ be a matroid, $c: E \rightarrow \mathbb{R}_{\geq 0}$,  $U \subseteq E$, $q \in \mathbb{N}$, and $B$ be a minimum basis of $[ \cG \cap U]_{\leq q}$ w.r.t. $c$. Also, let $\Delta \in \cI_{\leq q }$ and let $a \in (\Delta \cap U) \setminus B$. Then, there is $b \in B \setminus \Delta$ such that $\Delta - a+ b \in \cI$ and $c(b) \leq c(a)$.
\end{lemma}

\begin{proof}

Define $D = \{e \in B~|~c(e) \leq c(a)\}$ and let 
\begin{equation}
	\label{eq:I2q}
	\cI^U_{\leq q} = \{A \subseteq U~|~A \in \cI, |A| \leq q\}
\end{equation} be the collection of independent sets of the matroid $[\cG \cap U]_{\leq q}$ by Definition~\ref{def:matroids}. Note that $a \in  U \setminus B$; in addition, since $D \subseteq B$ and $a \notin B$ it holds that $a \notin D$. Therefore,  it follows that $D+a \notin \cI^U_{\leq q}$ by Lemma~\ref{lem:notIS}. We consider two cases. %We use the following auxiliary claim.%Thus, since $D,\Delta \in \cI_{\leq q(\eps)}$, $a \in \Delta \setminus D$ and  $D+a \notin \cI_{\leq q(\eps)}$, 

%	\begin{claim}
%	\label{claim:AUXsos}
%	 There is  $b \in D \setminus \Delta$ such that $\Delta-a+b \in \cI$. 
%\end{claim}
%\begin{claimproof}
  \begin{itemize}
		\item $D+a \in \cI$. Then, \begin{equation}
			\label{eq:DaI2}
			|D| \geq q \geq |\Delta|>|\Delta-a|.
		\end{equation} %By \eqref{eq:cj} it holds that $|D+a|>q(\eps) \geq |\Delta|>|W|$ 
		The first inequality holds since $D+a  \in \cI$, $D+a \notin \cI^U_{\leq q}$, and $D+a \subseteq U$; thus, $|D+a|> q$ by \eqref{eq:I2q}. The second inequality follows since $\Delta \in \cI_{\leq q }$ and the last inequality holds because $a \in \Delta$. %; it follows that $|D|> |W|$. 
		Observe that  by the hereditary property it holds that $D \in \cI^U_{\leq q} \subseteq \cI_{\leq q}$ and that $\Delta-a \in \cI_{\leq q}$ (note that $\Delta \in \cI_{\leq q}$). 
		Thus, by \eqref{eq:DaI2} and the exchange property of  $[\cG]_{\leq q}$ there is $b \in D \setminus (\Delta-a)$ such that $\Delta-a+b \in \cI_{\leq q}$. Because $a \notin D$ it holds that $b \notin \Delta$. It follows that $c(b) \leq c(a)$ using $b \in D$.
		
		\item $D+a \notin \cI$. Observe that $\Delta \in \cI$ by Definition~\ref{def:matroids}; also, observe that $D \in \cI$ because $D \subseteq B$, $ B \in \cI^U_{\leq q}$, and $\cI^U_{\leq q} \subseteq \cI$. Therefore, by Lemma~\ref{lem:gen} there is $b \in D \setminus \Delta$ such that $\Delta-a+b \in \cI_{\leq q}$. Observe that $c(b) \leq c(a)$ because $b \in D$. %Finally, because $b \in B_S$, then by Step~\ref{step:U_S} and Step~\ref{step:Br} of Algorithm~\ref{alg:representative} we have that $S+e \in \cI_{1}$. 
	\end{itemize}
%\end{claimproof}
\end{proof} 
\noindent{\bf Proof of Lemma~\ref{lem:Thereb}:} By Lemma~\ref{lem:NN} there is  $b \in B \setminus \Delta$ such that $\Delta-a+b \in \cI_{2}$ and $c(b) \leq c(a)$. Therefore, by Definition~\ref{def:shift} if it also holds that $\Delta-a+b \in \cI_{1}$, then $b$ is a shift to $a$ for $\Delta$; otherwise, $\Delta-a+b \notin \cI_{1}$ and it holds that $b$ is a semi-shift to $a$ for $\Delta$. \qed%The proof follows by Lemma~\ref{lem:NN} and Definition~\ref{def:shift}. 

% \qed%that $b \neq a$ since $b \in D, D \subseteq B, a \notin B$. \qed%and Step~\ref{step:Br} of Algorithm~\ref{alg:representative}. 

%

~\\

\noindent{\bf Proof of Lemma~\ref{claim:emptyChain}:}
	Let $S = \emptyset$. Trivially, $ \emptyset \subseteq X$ and $S \in \mathcal{S}$ by \eqref{eq:Ex-set}. Moreover, since $a \in \Delta$ and $\Delta \in \cm_{\leq q(\eps)}$, by the hereditary property $a = \emptyset+a \in \cI_1$; thus,  $a \in U_{\emptyset}$ by Step~\ref{step:U_S} of Algorithm~\ref{alg:representative}. Finally, for all $e \in \emptyset$ it holds that $e$ is a semi-shift to $a$ for $\Delta$ as a vacuous truth. Thus, $\emptyset$ is a chain of $a$ and $\Delta$ by Definition~\ref{def:chain}. \qed

~\\

\noindent{\bf Proof of Lemma~\ref{claim:qChain}:}
	Assume towards contradiction that $|S| > q(\eps)$; then, 
	\begin{equation}
		\label{eq:ddd}
		|S| > q(\eps) \geq |\Delta| > |\Delta-a|.
	\end{equation} 
	The second inequality holds since $\Delta \in \cm_{\leq q(\eps)}$. Now, by Definition~\ref{def:chain} $a \in U_{S}$, and by Step~\ref{step:U_S} of Algorithm~\ref{alg:representative} it holds that $S+a \in \cI_1$; therefore, $S \in \cI_1$. In addition, as $\Delta \in \cm_{\leq q(\eps)}$, by the hereditary property $\Delta -a \in \cI_{1}$. Therefore, by \eqref{eq:ddd} and the exchange property of $(E,\cI_{1})$ there is $e \in S \setminus (\Delta-a)$ such that $\Delta-a+e \in \cI_1$. However, as $S$ is a chain and $e \in S$, we have that $e$ is a semi-shift to $a$ for $\Delta$ (see Definitions~\ref{def:shift} and~\ref{def:chain}), implying that $\Delta-a+e \notin \cI_1$. Contradiction. \qed
~\\

\noindent{\bf Proof of Lemma~\ref{lem:maximum}:}
By Lemma~\ref{lem:Thereb}, there is $b^* \in B_{S^*}$ such that $b^*$ is a semi-shift or a shift to $a$ for $\Delta$. Assume towards a contradiction that $b^*$ is a semi-shift to $a$ for $\Delta$. We show that $S^*+b^*$ is a chain of $a$ and $\Delta$. 
\begin{itemize}
	\item $S^*+b^* \in \mathcal{S}$. Follows from Step~\ref{step:RBS} of Algorithm~\ref{alg:representative} and since $|S^*| \leq q(\eps)$, by Lemma~\ref{claim:qChain}.
	\item $a \in U_{S^*+b^*}$. Assume towards contradiction that $a \notin U_{S^*+b^*}$; then, by Lemma~\ref{lem:gen}, there is $e \in S^*+b^*$ such that $\Delta -a+e \in \cI_{1}$. Contradiction (as $S^*$ is a chain of $a$ and $\Delta$, and $b^*$ is a semi-shift to $a$ for $\Delta$).
	\item $\forall e \in S^*+b^*$ it holds that $e$ is a semi-shift to $a$ for $\Delta$. This follows since $S^*$ is a chain of $a$ and $\Delta$ and $b^*$ is a semi-shift to $a$ for $\Delta$, by our assumption. 
\end{itemize}
By the above, $S^*+b^*$ is a chain of $a$ and $\Delta$.
Furthermore, $|S^*+b^*| > |S^*|$ since $b^* \in B_{S^*}	\subseteq U_{S^*}$ and 
$B_{S^*} \cap S^* = \emptyset$. Thus, we have a contradiction to the maximality of $S^*$. We conclude that $b^*$ is a shift to $a$ for $\Delta$. \qed

~\\

\noindent{\bf Proof of Lemma~\ref{lem:mainMatroid}:} Let $\Delta \in \cm_{\leq q(\eps)}$, $a \in (C_r(\alpha) \cap \Delta) \setminus X$, %Let $\mathcal{F}$ be the set of all chains of $a$ and $\Delta$. In addition, let \begin{equation}
	%	\label{eq:argmax}
	%	S^* \in \left\{T \in \mathcal{F}~|~ |T| = \argmax_{S' \in \mathcal{F}} |S'|\right\}
	%	\end{equation} 
and let $S^*$ be a chain of $a$ and $\Delta$ of maximum cardinality. By Lemma~\ref{claim:emptyChain} there is some chain of $a$ and $\Delta$, and by Definition~\ref{def:chain} a chain is a finite subset of elements; thus, $S^*$ is well defined. By Lemma~\ref{claim:qChain} it holds that $|S^*| \leq q(\eps)$; thus, by Step~\ref{step:q} and Step~\ref{step:Br} of Algorithm~\ref{alg:representative}, and \eqref{eq:Ex-set}, it holds that $B_{S^*}$ is computed by Algorithm \textsf{ExSet-MatroidIntersection}. Then, %by Lemma~\ref{lem:Thereb} there is $b \in B_{S^*}$ such that $b$ is a semi-shift or a shift to $a$ for $\Delta$; by the maximality of $S^*$ it holds that 
by Lemma~\ref{lem:maximum} there is a shift $b^* \in B_{S^*}$ to $a$ for $\Delta$. %(otherwise $S^*+b$ is a chain of larger cardinality than $S^*$). 
Note that $B_{S^*} \subseteq X$ by Step~\ref{step:RBS} of Algorithm~\ref{alg:representative}. Therefore, by Definition~\ref{def:shift} (shift) and Definition~\ref{def:r-set} (exchange set) it follows that $X$ is an exchange set of $I,\eps,\alpha$, and $r$. We use the following claim for the complexity analysis. %; the proof is given in Appendix~\ref{sec:omitted-matroid}. 
	\begin{claim}
	\label{claim:r<4}
	$|X| \leq q(\eps)^{O(q(\eps)}$ and the running time of the algorithm is $q(\eps)^{O(q(\eps)} \cdot \textnormal{poly}(|I|)$.
\end{claim} 
\begin{claimproof}

		%Observe that the operations in each recursive call to Algorithm \textsf{ExtendChain} (i.e., without secondary recursive calls) can be computed in polynomial time in the instance size, as finding a minimum basis in Step~\ref{step:Br} can be done in linear time (see, e.g., \cite{cormen2022introduction}). %In addition,  for all $t \in \{0,\ldots, q(\eps)\}$, the iteration of $t$ of the {\bf while} loop can be computed in time $|L_t| \cdot x \cdot \textnormal{poly}(|I|)$ by Step~\ref{step:Lt} and that the computed bases are of sizes bounded by $q(\eps)$ by Definition~\ref{def:matroids}.

 Recall that $\mathcal{S}$ is the set of all branches $S \subseteq {\ck}_r(\alpha)$ such that $\textsf{ExtendChain}(I,\eps,\alpha,r,S)$ is computed during the execution of $\textsf{ExSet-MatroidIntersection}(I,\eps,\alpha,r)$. For all $t \in \{0,1,\ldots, q(\eps)+1\}$ let 
		$L_t = \{S \in \mathcal{S}~|~|S| = t\}$ % ~|~S = \{b_1, \ldots, b_t\}, \forall i \in [t]: b_i \in B_{b_1, \ldots, b_{i-1}}\}
		be the set of branches $S$ containing $t$ elements computed in some iteration of Step~\ref{step:Br} of Algorithm~\ref{alg:representative} in the course of Algorithm \textsf{ExSet-MatroidIntersection}. 	Observe that the operations in each recursive call to Algorithm \textsf{ExtendChain} (i.e., without secondary recursive calls) can be computed in polynomial time in the instance size, as finding a minimum basis in Step~\ref{step:Br} can be done in linear time (see, e.g., \cite{cormen2022introduction}). Moreover, by Step~\ref{step:RBS} and Step~\ref{step:q}, the number of recursive calls to the algorithm is bounded by the number of branches reached by the algorithm. Note that the branches are of sizes between $0$ and $q(\eps)+1$ by \eqref{eq:Ex-set} and Step~\ref{step:q} of Algorithm~\ref{alg:representative}. 	In addition, each branch $S$ induces $|S|$ recursive calls to Algorithm~\ref{alg:representative}. Thus, the running time of the algorithm can be bounded by \begin{equation}
		\label{eq:1111}
		\begin{aligned}
		\sum_{t \in \{0,1,\ldots, q(\eps)+1\}} \sum_{S \in L_t} |B_S| \cdot \textnormal{poly}(|I|) \leq{} & 	\sum_{t \in \{0,1,\ldots, q(\eps)+1\}} |L_t| \cdot q(\eps) \cdot \textnormal{poly}(|I|)\\
		\leq{} & (q(\eps)+1) \cdot {q(\eps)}^{q(\eps)+1} \cdot q(\eps) \cdot  \textnormal{poly}(|I|)\\
		 = {}& q(\eps)^{O(q(\eps)} \cdot \textnormal{poly}(|I|). 
		\end{aligned}
	\end{equation} The first inequality holds since for every branch $S$ it holds that $|B_S| \leq q(\eps)$ by Step~\ref{step:Br} and Definition~\ref{def:matroids}. 	The second inequality holds since $\forall t \in [q(\eps)]: |L_{t+1}| \leq q(\eps) \cdot |L_t|$ by Step~\ref{step:RBS} of Algorithm~\ref{alg:representative}; thus, as $|L_0|  = 1$ by \eqref{eq:Ex-set}, by an inductive argument it holds that $\forall t \in [q(\eps)+1]: |L_t| \leq q(\eps)^{q(\eps)+1}$. %The last equality follows by Claim~\ref{claim:RSize}. The running time of Algorithm \textsf{Exset-MatroidIntersection} is bounded by $q(\eps)^{O(q(\eps))} \cdot \textnormal{poly}(|I|)$. 
Finally, for the size of $X$, the returned exchange set, we have	\begin{equation*}
		\label{eq:lastanalysis}
		\begin{aligned}
			|X| ={} & \left|\bigcup_{t \in \{0,1,\ldots, q(\eps)+1\}} \bigcup_{S \in L_t} B_S\right| \\
			\leq{} & \sum_{t \in \{0,1,\ldots, q(\eps)+1\}} \sum_{S \in L_t} |B_S| \\
			\leq{} & \sum_{t \in \{0,1,\ldots, q(\eps)\}} |L_t| \cdot q(\eps)  \\
			= {} & q(\eps)^{O(q(\eps))}.
		\end{aligned}
	\end{equation*} The first equality holds by \eqref{eq:Ex-set}, and Steps~\ref{step:q},~\ref{step:RBS} of Algorithm~\ref{alg:representative}. The second inequality holds by Step~\ref{step:Br}, since the computed bases $B_S$ are of sizes bounded by $q(\eps)$ by Definition~\ref{def:matroids}. The last inequality holds by symetric arguments to \eqref{eq:1111}. %The second equality follows by Claim~\ref{claim:RSize}. The last equality follows by \eqref{eq:rrr}. 
\end{claimproof}
The proof of Lemma~\ref{lem:mainMatroid} follows by the above.  \qed
